# Supplementary material for: AI-based Aortic Vessel Tree Segmentation for Cardiovascular Diseases Treatment: Status Quo
Source: arXiv:2108.02998 source file (2023-04-03)
Supplement: Supplementary file 1 [file SUPPLEMENTARY.pdf]

# SUPPLEMENTARY MATERIAL

## Flow Diagram

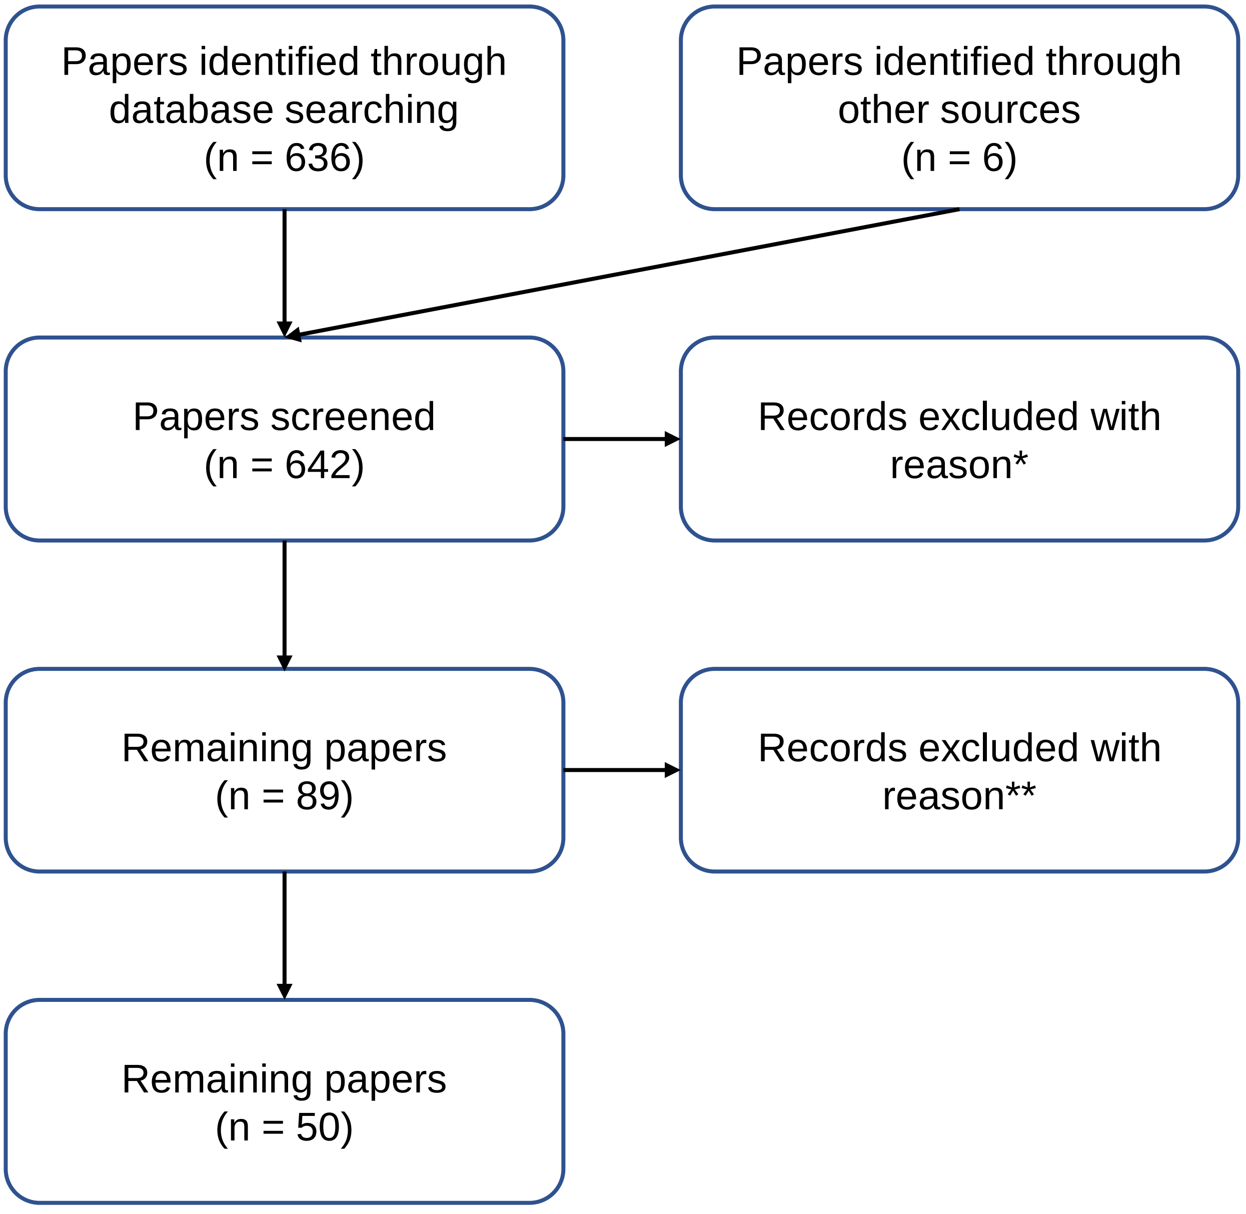


*The reason for exclusion was for example a pure clinical contribution of the article, such as aorta measurements and medical findings.

** The reason for exclusion was the overlap of contents with other papers or the lack of quantitative segmentation results.

SEARCH ENGINES:
IEEE Xplore, PubMed, Google Scholar and ScienceDirect

Keywords:
‘aorta’ AND ‘segmentation’ [Title/Abstract]

Date of search: March 2021

**IEEE Xplore: 152**
**PubMed: 282**
**Google Scholar*: 104**
**ScienceDirect: 98**

**TOTAL: 636**

*Differently than other engines, Google Scholar also searches in text and references. Therefore, only in this specific case, each search was filtered with the operator ‘allintitle’, e.g., allintitle: aorta segmentation.

## DATABASE OVERLAP

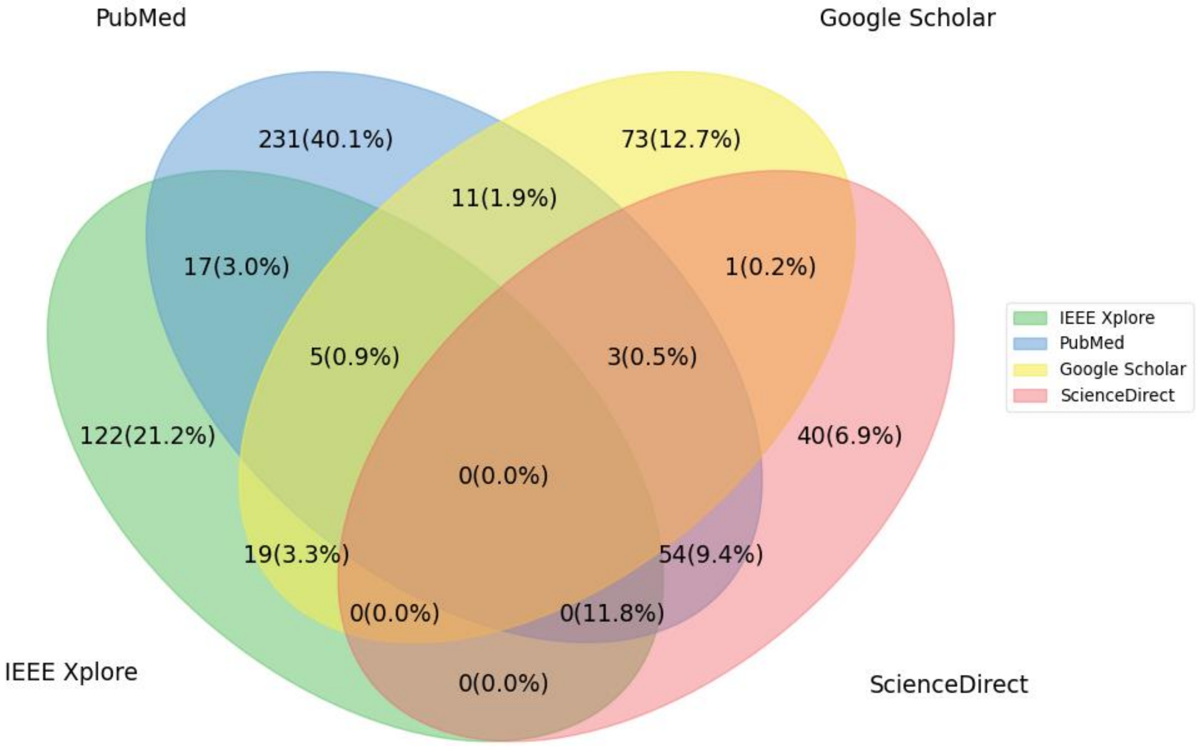


**Overall distribution after screening of the articles retrieved from the four databases and relative overlapping**.
